# Supplementary material for: One cut, two parities: exact Fibonacci charge responses in the golden chain
Source: arXiv:2607.01151 source file (2026-09-01)
Supplement: Supplementary file 1 [file supplement.tex]

% ===== Supplemental Material: PRL =====
\onecolumngrid
\clearpage

\begin{center}
  {\large\bfseries Supplemental Material}
\end{center}

\setcounter{section}{0}
\setcounter{equation}{0}
\setcounter{figure}{0}
\setcounter{table}{0}

\setcounter{secnumdepth}{3}

This Supplemental Material collects the technical details underlying the
main text: the exact fusion-path superselection structure
(Sec.~S1), the complete proof of the finite-size cut-charge theorem for
the even-length Fibonacci chain (Sec.~S2), the rank-3
$\mathrm{su}(2)_5$ modular-data benchmark (Sec.~S3), and the direct
finite-size numerical verification of the sandwiched-projector identity
(Sec.~S4).  Equation and section numbers are prefixed by ``S''; references
to unprefixed numbers refer to the main text.

\section*{Cut-charge theorem: complete proof}

\subsection{Fusion-path basis and exact superselection}

The Hilbert space $\mathcal V^{(\tau)}$ is the Fibonacci fusion-path space
with a single $\tau$-insertion. Each basis state is an admissible height
string $|h_0,\ldots,h_{L-1}\rangle$ in the A4 RSOS representation. A
spatial bipartition cuts the chain at an internal bond $\ell$, which
carries a definite anyon charge $a_\ell\in\{\mathbf 1,\tau\}$. The reduced
density matrix of the left half is exactly block diagonal in that charge,
\begin{equation}
\rho_A = \bigoplus_{a\in\{\mathbf 1,\tau\}} \rho_A^{(a)},
\qquad
P_a \equiv \mathrm{Tr}\,\rho_A^{(a)} = \sum_{k:\,c_k=a} \lambda_k^2,
\label{eq:sm-blockdiag}
\end{equation}
where $\{\lambda_k^2\}$ are Schmidt weights and $c_k$ is the cut charge.

\subsection{Two-charge theorem proof}

Let $\Omega_L$ be the nondegenerate AFM ground state for even $L$.
The topological symmetry operator $Y_\tau$ acts on the fusion-path
basis by inserting a $\tau$-loop around the chain. Its possible
eigenvalues are $\varphi$ and $-1/\varphi$, as follows from the
Fibonacci Verlinde formula $S_{\tau a}/S_{\mathbf 1 a}=d_a$. The point of
Step~1 is to determine which of these two topological sectors contains
the even-$L$ AFM ground state.

\emph{Step 1: Ground-state eigenvalue.}
The Hamiltonian $H=-\varphi\sum_i P_i$ with
$P_i=e_i/\varphi$ is stoquastic: all off-diagonal matrix elements are
non-positive in the fusion-path basis, because the local Temperley--Lieb
projector $P_i$ has matrix elements
$(A_4\,\textrm{RSOS})$ only connecting admissible height configurations
and carries a single-channel expansion in the Fibonacci planar algebra.
The representation is irreducible for even $L$: the periodic
fusion-path space $\mathcal V^{(\tau)}$ is a single connected graph under
the action of $H$, because the TL algebra generated by $\{e_i\}$ at
$\delta=\varphi$ acts transitively on height configurations compatible
with the single $\tau$-insertion~\cite{Feiguin2007golden,GilsArdonne2013}.
Perron--Frobenius therefore gives a unique ground
state with strictly positive coefficients in the fusion-path basis. The topological symmetry
$Y_\tau$ commutes with $H$, so this state lies entirely in either the
$Y_\tau=\varphi$ sector or the $Y_\tau=-1/\varphi$ sector.

To select the sector, let $|T\rangle=|\tau\tau\cdots\tau\rangle$ and
consider $u=E_+|T\rangle$. We spell out the sign input. In the gauge used in the Letter, the
nontrivial Fibonacci block has entries
$\varphi^{-1},\varphi^{-1/2},\varphi^{-1/2},-\varphi^{-1}$; the only
negative entry is the $\tau\tau\to\tau\tau$ channel. In the cyclic
hoop matrix element from the all-$\tau$ path to an output path $y$, all
nonzero local factors are therefore positive except one factor
$-\varphi^{-1}$ for each adjacent $\tau\tau$ pair in $y$. Hence
\begin{equation}
\operatorname{sgn}\langle y|Y_\tau|T\rangle
=(-1)^{N_{\tau\tau}(y)},
\end{equation}
where $N_{\tau\tau}(y)$ is the number of adjacent $\tau\tau$ pairs.
Because admissible Fibonacci paths have no adjacent vacuum labels, each
vacuum label removes two adjacent $\tau\tau$ pairs from the all-$\tau$
cycle, so $N_{\tau\tau}(y)=L-2z(y)$ with $z(y)$ the number of vacuum
labels. Thus for even $L$ every nonzero hoop contribution to
$E_+|T\rangle=(|T\rangle+\varphi Y_\tau|T\rangle)/D^2$ has positive
sign, and the all-$\tau$ component is nonzero. Therefore $u$ is a
nonzero componentwise nonnegative vector. A positive Perron--Frobenius
ground state has positive overlap with this vector; hence it cannot lie
in the orthogonal $E_-$ sector.
Therefore
\begin{equation}
E_+\Omega_L=\Omega_L,
\qquad
Y_\tau\Omega_L=\varphi\Omega_L .
\label{eq:sm-ground-sector}
\end{equation}
For odd $L$ the parity in the same sign calculation is reversed, so the
above positivity witness no longer selects the $E_+$ ground-state sector.
Accordingly the finite-ground-state statement in the Letter is restricted
to even $L$. We do not use, or claim, an automatic $E_-$ replacement of
Eq.~\eqref{eq:sm-sandwiched}: replacing $E_+$ by the complementary
projector changes both the relevant block normalization and the rank input,
so it would require a separate finite-size sector analysis rather than a
formal substitution.

\emph{Step 2: Sandwiched projector identity.} This step is an operator
identity on the periodic path space and does not use the ground state.
Fix the cut and decompose
\begin{equation}
\mathcal H_L=\mathcal H_{\mathbf1}\oplus\mathcal H_\tau,
\qquad
\mathcal H_a=\Pi_a^{(\ell)}\mathcal H_L .
\end{equation}
Set
\begin{equation}
A=I+\varphi Y_\tau=D^2E_+ .
\end{equation}
The local Fibonacci fusion rule gives the $\mathbf1\mathbf1$ block
$(Y_\tau)_{\mathbf1\mathbf1}=0$: a single $\tau$ hoop crossing a vacuum
cut changes the cut channel to $\tau$ and cannot return to vacuum.
Hence
\begin{equation}
A_{\mathbf1\mathbf1}=I .
\label{eq:sm-A00}
\end{equation}

It remains to know the rank of $E_+$. Let
$N=\bigl(\begin{smallmatrix}0&1\\1&1\end{smallmatrix}\bigr)$ be the
Fibonacci fusion adjacency matrix. Then
\begin{equation}
\dim\mathcal H_L=\mathrm{Tr}(N^L),
\qquad
\dim\mathcal H_{\mathbf1}=(N^L)_{\mathbf1\mathbf1} .
\end{equation}
The cyclic $F$-symbol formula for $Y_\tau$ gives
\begin{equation}
\mathrm{Tr}(Y_\tau)=(-1/\varphi)^L .
\label{eq:sm-traceY}
\end{equation}
A direct verification: the matrix elements of $Y_\tau$ in the
fusion-path basis are
\begin{equation}
\langle y|Y_\tau|x\rangle
=\prod_{i=0}^{L-1}
F^{\tau\,x_{i+1}\,y_i}_{x_i\,y_{i+1}},
\qquad
x_L\equiv x_0,\; y_L\equiv y_0,
\end{equation}
where $F$ is the Fibonacci $F$-symbol used in the main text and indices
run over $\{\mathbf1,\tau\}$. For the diagonal $y=x$, the local factor
$F^{\tau\,x_{i+1}\,x_i}_{x_i\,x_{i+1}}$ vanishes unless
$x_i=x_{i+1}=\tau$: a $\mathbf1\to\tau\to\mathbf1$ or
$\mathbf1\to\mathbf1\to\mathbf1$ local loop has zero amplitude in the
Fibonacci $F$-symbol. The only surviving diagonal path is the
all-$\tau$ configuration $x=(\tau,\tau,\dots,\tau)$, for which each
local factor equals $F^{\tau\tau\tau}_\tau=-1/\varphi$. Multiplying $L$
identical factors gives Eq.~\eqref{eq:sm-traceY}. Since $E_+$ is an
orthogonal projection,
\begin{equation}
\mathrm{rank}(E_+)=\mathrm{Tr}(E_+)
=\frac{\mathrm{Tr}(N^L)+\varphi(-1/\varphi)^L}{D^2}
=(N^L)_{\mathbf1\mathbf1}
=\dim\mathcal H_{\mathbf1},
\label{eq:sm-rank}
\end{equation}
where the penultimate equality follows by diagonalizing $N$, whose
eigenvalues are $\varphi$ and $-1/\varphi$. This rank computation uses
only the cyclic trace of $Y_\tau$ and the Fibonacci path-counting matrix;
it is independent of the sandwiched-projector identity that follows.

Now we extract the block structure of $A$ from the two inputs
Eqs.~\eqref{eq:sm-A00} and \eqref{eq:sm-rank}.

\emph{Lemma (Projection graph lemma).}
Let $P$ be an orthogonal projection on $\mathcal H_{\mathbf1}\oplus\mathcal H_\tau$
and set $A=D^2P$ with $D^2=1+\varphi^2$. If
\begin{equation}
A_{\mathbf1\mathbf1}=I_{\mathcal H_{\mathbf1}},\qquad
\mathrm{rank}(A)=\dim\mathcal H_{\mathbf1},
\label{eq:sm-lemma-hyp}
\end{equation}
then $\mathrm{Ran}(P)$ is the graph of a linear map
$T:\mathcal H_{\mathbf1}\to\mathcal H_\tau$ satisfying
$T^\dagger T=\varphi^2I$, i.e.\ $T=\varphi V$ with $V$ an isometry.
Equivalently
\begin{equation}
A=\begin{pmatrix}
I & \varphi V^\dagger\\
\varphi V & \varphi^2VV^\dagger
\end{pmatrix} .
\label{eq:sm-graph}
\end{equation}

\emph{Proof of the lemma.}
Let $S=\mathrm{Ran}(P)$ and let $\pi_{\mathbf1}$ denote orthogonal
projection from $\mathcal H_{\mathbf1}\oplus\mathcal H_\tau$ onto
$\mathcal H_{\mathbf1}$. The hypothesis gives
$\dim S=\mathrm{rank}(P)=\mathrm{rank}(A)=\dim\mathcal H_{\mathbf1}$ and
\begin{equation}
P_{\mathbf1\mathbf1}
=\pi_{\mathbf1}P\pi_{\mathbf1}^\dagger
=\frac{1}{D^2}I_{\mathcal H_{\mathbf1}} .
\end{equation}
Equivalently, for the map $Q:S\to\mathcal H_{\mathbf1}$ obtained by
restricting $\pi_{\mathbf1}$ to $S$, one has
$QQ^\dagger=I/D^2$. Thus $Q$ is surjective; since its domain and codomain
have the same finite dimension, $Q$ is bijective. Hence every
$x\in\mathcal H_{\mathbf1}$ has a unique lift in $S$, so $S$ is the graph
of a unique linear map $T:\mathcal H_{\mathbf1}\to\mathcal H_\tau$:
\begin{equation}
\mathrm{Ran}(P)=\{(x,Tx):x\in\mathcal H_{\mathbf1}\}.
\end{equation}
The orthogonal projector onto a graph has the standard block form
\begin{equation}
P_{\rm graph}=
\begin{pmatrix}
(I+T^\dagger T)^{-1} & (I+T^\dagger T)^{-1}T^\dagger\\
T(I+T^\dagger T)^{-1} & T(I+T^\dagger T)^{-1}T^\dagger
\end{pmatrix} .
\label{eq:sm-graph-form}
\end{equation}
Equating $P_{\mathbf1\mathbf1}=I/D^2$ with the top-left block of
Eq.~\eqref{eq:sm-graph-form} gives $(I+T^\dagger T)^{-1}=I/D^2$,
hence $T^\dagger T=(D^2-1)I=\varphi^2I$. Therefore $T=\varphi V$
with $V^\dagger V=I$. Substituting into Eq.~\eqref{eq:sm-graph-form}
and multiplying by $D^2$ yields Eq.~\eqref{eq:sm-graph}.
$\square$

\emph{Compact algebraic alternative.}
The block form can also be read directly from $A^2=D^2A$, which follows
from $A=I+\varphi Y_\tau$, $Y_\tau^2=I+Y_\tau$, and $\varphi^2=\varphi+1$:
\begin{equation}
A^2=I+2\varphi Y_\tau+\varphi^2Y_\tau^2
=I+2\varphi Y_\tau+\varphi^2(I+Y_\tau)=D^2(I+\varphi Y_\tau)=D^2A.
\label{eq:sm-A2check}
\end{equation}
Write $A$ in block form
$A=\bigl(\begin{smallmatrix}I&B^\dagger\\B&C\end{smallmatrix}\bigr)$,
where $B:\mathcal H_{\mathbf1}\to\mathcal H_\tau$, with
$A_{\mathbf1\mathbf1}=I$ from Eq.~\eqref{eq:sm-A00}.
The $(1,1)$ block of $A^2=D^2A$ gives
$I+B^\dagger B=D^2I$, hence $B^\dagger B=\varphi^2I$.
By singular-value decomposition $B=\varphi V$ with $V^\dagger V=I$.
Since $A\ge0$ and $A_{\mathbf1\mathbf1}=I$ has full rank, the Schur
complement of $A$ vanishes: $C=BB^\dagger$.
Thus $C=(\varphi V)(\varphi V^\dagger)=\varphi^2VV^\dagger$, recovering
Eq.~\eqref{eq:sm-graph}.
This algebraic path is independent of the graph-projection lemma;
the two derivations cross-check each other.

Applying this lemma with
$P=E_+$ and $A=D^2E_+$, the block form
Eq.~\eqref{eq:sm-graph} follows directly from
Eqs.~\eqref{eq:sm-A00} and \eqref{eq:sm-rank}.
Therefore
\begin{equation}
A\Pi_{\mathbf1}^{(\ell)}A=A,
\qquad
A\Pi_\tau^{(\ell)}A=A^2-A=(D^2-1)A=\varphi^2A .
\end{equation}
Dividing by $D^4$ proves
\begin{equation}
E_+\Pi_{\mathbf1}^{(\ell)}E_+=\frac{1}{D^2}E_+,
\qquad
E_+\Pi_\tau^{(\ell)}E_+=\frac{\varphi^2}{D^2}E_+ .
\label{eq:sm-sandwiched}
\end{equation}
This is the advertised sandwiched identity. Equivalently, the block form
above says that the overlap between the vacuum-tube subspace $E_+\mathcal H_L$
and the cut-charge subspace $\mathcal H_{\mathbf1}$ is a scalar isometry:
all nonzero singular values of $E_+\Pi_{\mathbf1}^{(\ell)}$ are exactly
$1/D$. Thus the tube-flux and cut-charge resolutions are crossed bases
inside the vacuum sector. Notice that no commutation of
$\Pi_a^{(\ell)}$ with $H$ or $Y_\tau$ is assumed; in fact the
unsandwiched and commutator versions are false.

\emph{Step 3: Sector weights and $g$-function.}
Taking the expectation in the even-$L$ ground state and using
Eq.~\eqref{eq:sm-ground-sector},
\begin{align}
P_a
&=\langle\Omega_L|\Pi_a^{(\ell)}|\Omega_L\rangle
 =\langle\Omega_L|E_+\Pi_a^{(\ell)}E_+|\Omega_L\rangle\nonumber\\
&=\frac{d_a^2}{D^2}\langle\Omega_L|E_+|\Omega_L\rangle
 =\frac{d_a^2}{D^2} .
\end{align}
Hence $P_\tau/P_{\mathbf1}=\varphi^2$ and
$\ln g=\frac12\ln(P_\tau/P_{\mathbf1})=\ln\varphi$.

\subsection{\texorpdfstring{Rank-3 numerical benchmark: $\mathrm{su}(2)_5$ integer sector}{Rank-3 numerical benchmark: su(2)5 integer sector}}
\label{sec:sm-su25}

The finite-size proof above uses only Fibonacci fusion data plus the
Hamiltonian input that the ground state lies in the $Y_\tau=\varphi$
sector. A useful higher-rank benchmark is the integer sector
$a\in\{0,1,2\}$ of $\mathrm{su}(2)_5$. Its normalized restricted
modular matrix is
\begin{equation}
S_{ab}=\sqrt{\frac{4}{7}}\sin\frac{\pi(2a+1)(2b+1)}{7} .
\end{equation}
For the $a=1$ Verlinde defect, the sector eigenvalues are
$\lambda_b=S_{1b}/S_{0b}$. Thus the predicted polarization ratios are
\begin{equation}
r_b=|\lambda_b|^2:
\qquad
r_0=d_1^2,
\quad
r_1=\left(\frac{d_2}{d_1}\right)^2,
\quad
r_2=\frac{1}{d_2^2},
\label{eq:sm-su25-ratios}
\end{equation}
where
$d_1=\sin(3\pi/7)/\sin(\pi/7)=2.24698\ldots$ and
$d_2=\sin(5\pi/7)/\sin(\pi/7)=1.80194\ldots$.
Numerically,
\begin{equation}
(r_0,r_1,r_2)=(5.0489\ldots,0.6431\ldots,0.3080\ldots).
\end{equation}
The same ratios are implemented in the numerical benchmark script
\texttt{su2\_5\_verlinde\_ratios.jl}, which checks the normalized restricted
$S$ matrix and prints the three Verlinde polarization ratios.
This rank-3 pattern is not a Fibonacci identity in disguise: it has
three distinct polarization values fixed by the modular $S$ matrix.
The benchmark is included as category-level support and a numerical
target audit; the Letter proves the exact finite-lattice
sandwiched-projector theorem for the Fibonacci chain.

\subsection{Numerical verification}

A Julia script constructs the finite periodic Fibonacci path basis and the
matrix representation of $Y_\tau$ for $L=8,10,12,14$, then evaluates the
finite-dimensional operator identities for $E_+\Pi_a^{(\ell)}E_+$ directly.
All residuals are $<10^{-14}$. Code:
\texttt{verify\_sandwiched\_projector\_identity\_2026\_06\_24.jl} in the
reproducibility package.
